# Supplementary material for: Limiting Lamport Exposure to Distant Failures in Globally-Managed Distributed Systems
Source: arXiv:1405.0637 source file (2022-07-15)
Supplement: Supplementary file 1 [file appendix.tex]

\appendix
\label{sec:appendix}

\section{Appendix}

\subsection{Scalability analysis}

We study the system's scalability when the number of nodes increases.  We 
ask
two questions: (1)\say{\textit{How many zones / configuration services 
should a
		node expect to run?}}; and (2) \say{\textit{How much load should a 
		node expect
		when running x zones?}}. Fig~\ref{fig:theory-instances} answers the 
		first
question, depicting A CDF of the expected number of zones per node. We 
analyzed
different N and K parameters for a fixed network diameter. The fixed 
overhead,
\eg memory, increases linearly per additional zone the node runs.  But the
dynamic load depends on how many other nodes are running the same 
zone, because
only participating nodes impose load on the zone.
Fig~\ref{fig:theory-load} depicts the expected dynamic load per node per
node compared to the expected total number of zones in \name.  The   
network
diameter D is 128 ms and each node issues 100 requests. For a set of N, K 
and
D, the expected number of zones is uniquely determined; the experiment
varies N and plots the expected load per node for systems with parameter K 
= 2
to K = 5. The analysis shows that, with bigger networks and more zones, the
cost for each node grows with a slow logarithmic rate, which flattens for
bigger Ks. We conclude that \name scales well on large wide-area systems. 

\begin{figure}[h]                                                             
	\centering                                                                  
	\begin{subfigure}[t]{.22\textwidth}                                         
		\includegraphics[width=1.0\textwidth]{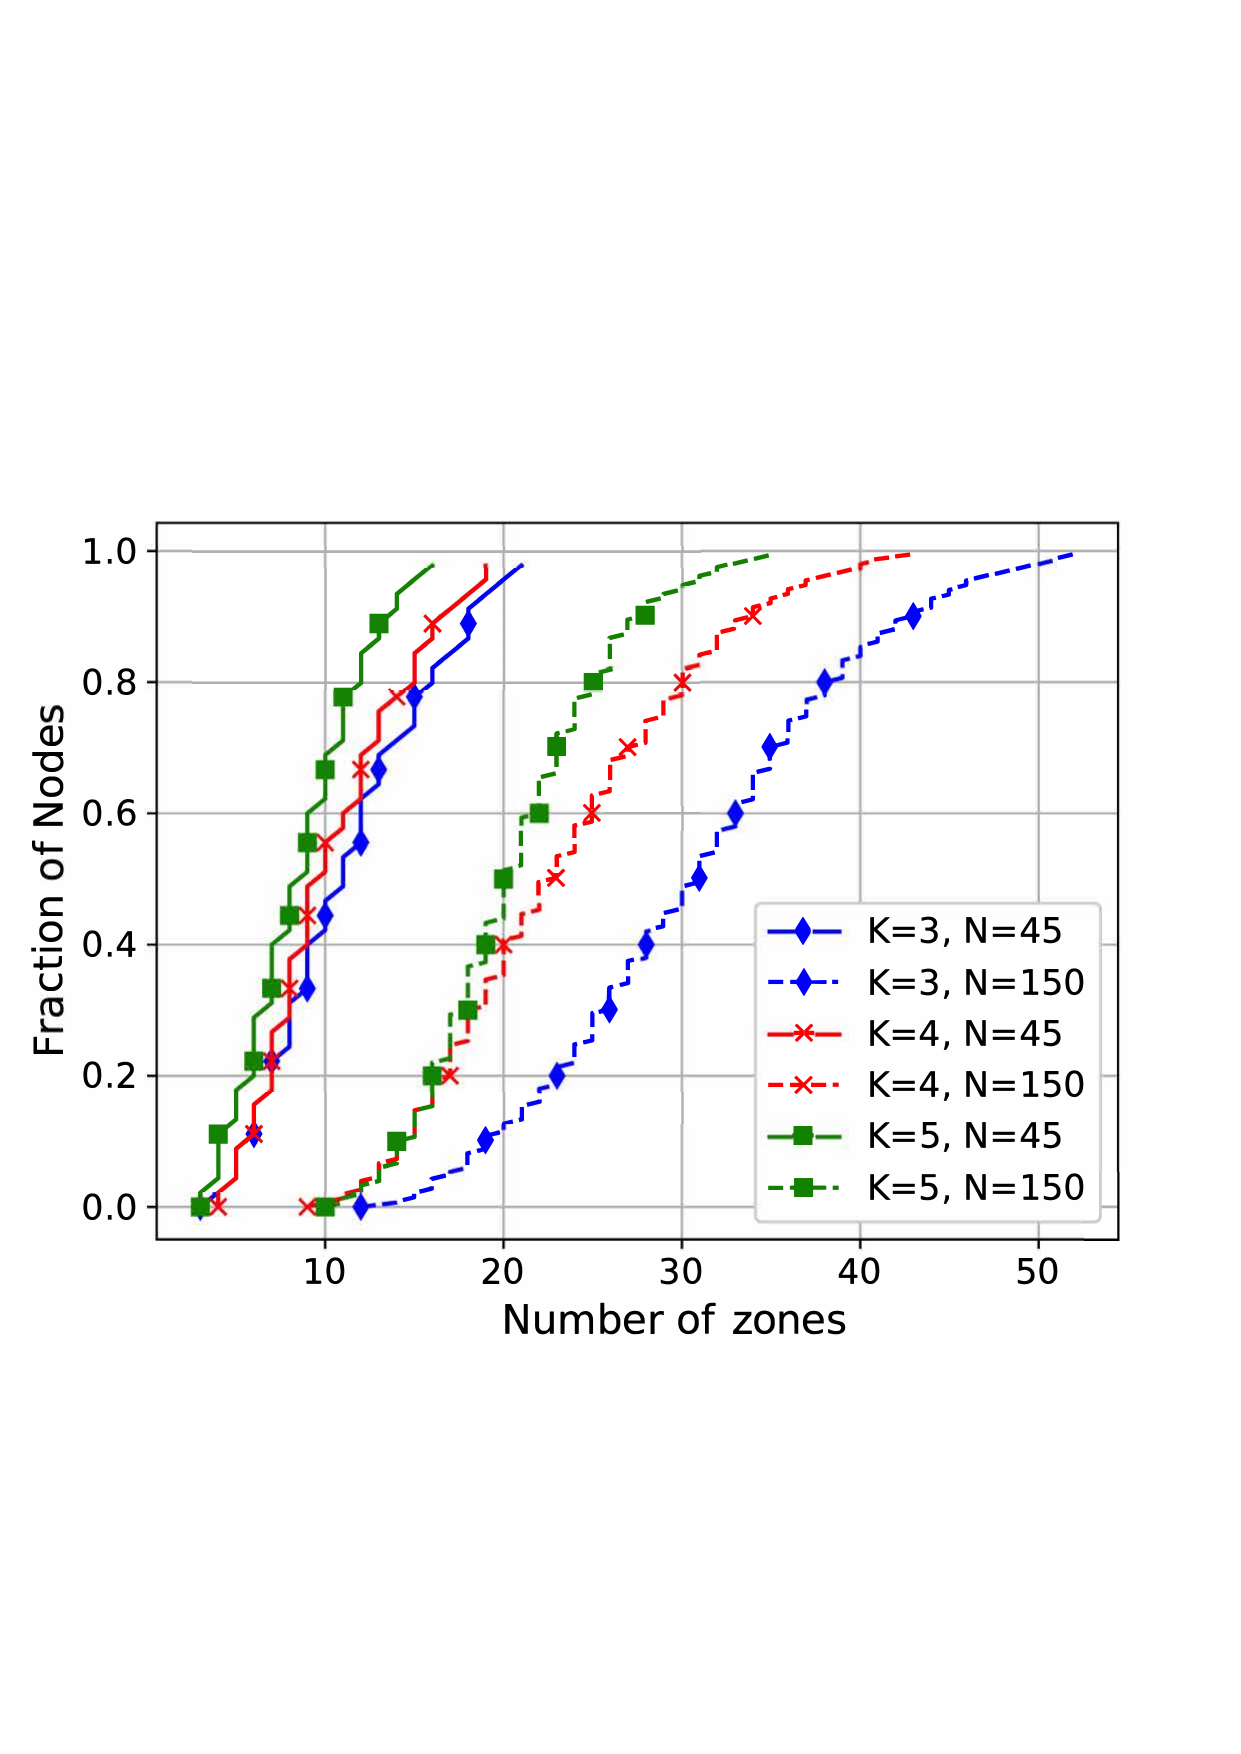}            
		\caption{Nr. of zones per zone.}                                        
		\label{fig:theory-instances}                                            
	\end{subfigure}\hfill                                                       
	\hspace{-0.2cm}                                                             
	\begin{subfigure}[t]{.26\textwidth}                                         
		\includegraphics[width=1.0\textwidth]{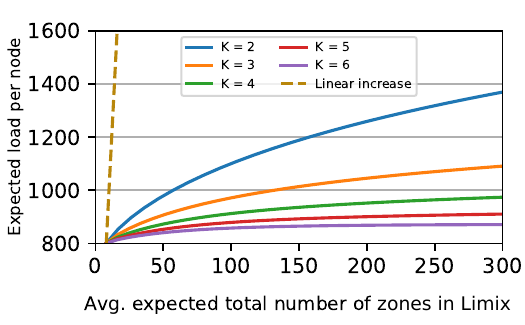}
		\caption{Exp. dynamic load per node.}                                   
		\label{fig:theory-load}                                                 
	\end{subfigure}\hfill                                                       
	\captionsetup{justification=centering}                                      
	\vspace{-0.2cm}                                                              
	\caption{Theoretical analysis: costs per node.}                             
	\vspace{-0.5cm}                                                              
\end{figure}
